# Supplementary material for: Heterogeneous node copying from hidden network structure
Source: arXiv:2102.09489 source file (2021-07-24)
Supplement: Supplementary file 1 [file Inner_Circle_Paper_PRL_Supplement__1_.pdf]

# Supplement: Correlated copying in a hidden network model

Max Falkenberg, *et al.*

Centre for Complexity Science, Imperial College London, SW7 2AZ, U.K.

## 1 Observed network second moment

Here we calculate the second moment for the observed network,  $\langle k_O^2 \rangle$ . First, we recall that

$$(k_O)_\alpha = \sum_{\beta=1}^{(k_H)_\alpha} (k_H)_{\alpha,\beta}. \quad (1.1)$$

Let us square both sides, and average over all nodes in the network such that

$$\frac{1}{t} \sum_{\alpha=1}^t (k_O)_\alpha^2 = \frac{1}{t} \sum_{\alpha=1}^t \left[ \sum_{\beta=1}^{(k_H)_\alpha} (k_H)_{\alpha,\beta} \right]^2. \quad (1.2)$$

We now simplify the left hand side and expand the squared sum on the right hand side to give

$$\langle k_O^2 \rangle = \frac{1}{t} \sum_{\alpha=1}^t \left[ \sum_{\beta=1}^{(k_H)_\alpha} (k_H)_{\alpha,\beta}^2 + \sum_{\beta=1}^{(k_H)_\alpha} \sum_{\beta' \neq \beta}^{(k_H)_\alpha} (k_H)_{\alpha,\beta} (k_H)_{\alpha,\beta'} \right], \quad (1.3)$$

where the first term in the brackets is the contribution from the product of node  $\alpha, \beta$  with itself, and the second term considers the cross term contribution between node  $\alpha, \beta$  and all other neighbors  $\alpha, \beta'$ . Taking the first term out of the brackets and summing over all nodes in the network gives

$$\langle k_O^2 \rangle = \langle k_H^3 \rangle + \frac{1}{t} \sum_{\alpha=1}^t \sum_{\beta=1}^{(k_H)_\alpha} \sum_{\beta' \neq \beta}^{(k_H)_\alpha} (k_H)_{\alpha,\beta} (k_H)_{\alpha,\beta'}, \quad (1.4)$$

where we have used the property that node  $\ell$  appears in the expanded sum  $(k_H)_\ell$  times. We proceed with a mean-field approximation and assume that as  $t \rightarrow \infty$  the average degree of next-nearest neighbors in the hidden network are uncorrelated. This implies that  $(k_H)_{\alpha,\beta}$  and  $(k_H)_{\alpha,\beta'}$  are uncorrelated. Hence, we can replace the sum over  $\beta'$  with  $(k_H)_\alpha - 1$  times the average degree of node  $(k_H)_{\alpha,\beta'}$  giving

$$\langle k_O^2 \rangle \approx \langle k_H^3 \rangle + \frac{1}{t} \sum_{\alpha=1}^t \sum_{\beta=1}^{(k_H)_\alpha} (k_H)_{\alpha,\beta} \langle k_H \rangle_{\alpha,\beta'} \cdot ((k_H)_\alpha - 1). \quad (1.5)$$

We know that due to the friendship paradox  $\langle k_H \rangle_{\alpha,\beta'} \neq \langle k_H \rangle$ . On average our friends have more friends than we do. For a network with zero assortativity, we can relate the average nearest neighbour degree to the average degree by

$$\langle k_H \rangle_{\alpha,\beta'} = \langle k_H \rangle + \frac{\sigma^2(k_H)}{\langle k_H \rangle}, \quad (1.6)$$

where  $\sigma^2$  is the degree variance. In our case this gives

$$\langle k_H \rangle_{\alpha,\beta'} = \langle k_H \rangle + \frac{\langle k_H^2 \rangle - \langle k_H \rangle^2}{\langle k_H \rangle} = 3. \quad (1.7)$$

Subbing this into Eq. (1.5) and rearranging slightly we can write

$$\langle k_O^2 \rangle \approx \langle k_H^3 \rangle + \frac{3}{t} \sum_{\alpha=1}^t \sum_{\beta=1}^{(k_H)_\alpha} [(k_H)_{\alpha,\beta} (k_H)_\alpha - (k_H)_{\alpha,\beta}], \quad (1.8)$$

where again we have a cross term between node  $\alpha, \beta$  and node  $\alpha$ . Hence, since the inner sum does not act on node  $\alpha$ , we also assume that the  $(k_H)_\alpha$  term can be replaced by Eq. (1.5) such that

$$\langle k_O^2 \rangle \approx \langle k_H^3 \rangle + \frac{3}{t} \sum_{\alpha=1}^t \sum_{\beta=1}^{(k_H)_\alpha} [3(k_H)_{\alpha,\beta} - (k_H)_{\alpha,\beta}] = \langle k_H^3 \rangle + \frac{6}{t} \sum_{\alpha=1}^t \sum_{\beta=1}^{(k_H)_\alpha} (k_H)_{\alpha,\beta}. \quad (1.9)$$

Finally, noting that each  $(k_H)_{\alpha,\beta}$  term appears exactly  $(k_H)_{\alpha,\beta}$  times in the expanded sum we find

$$\langle k_O^2 \rangle \approx \langle k_H^3 \rangle + 6\langle k_H^2 \rangle = 62, \quad (1.10)$$

where in the final line we have used  $\langle k_H^3 \rangle = 26$  and  $\langle k_H^2 \rangle = 6$ , both of which follow directly from the hidden degree distribution,  $p_H(k_H) = 2^{-k_H}$ . This result is consistent with direct measurements taken in simulations.

## 2 Observed degree distribution

### 2.1 Master Equation

The hidden network evolves as a random recursive tree which has a limiting degree distribution given by

$$p_H(k_H) = 2^{-k_H}, \text{ for } k > 1. \quad (2.1)$$

For the observed network we start with the master equation

$$\begin{aligned} N(t+1) \cdot p_O(k_O, t+1) - N(t) \cdot p_O(k_O, t) = \\ N(t) \cdot \Pi_O(k_O - 1, t) \cdot p_O(k_O - 1, t) - N(t) \cdot \Pi_O(k_O, t) \cdot p_O(k_O, t) + 2^{1-k_O}, \text{ for } k \geq 2, \end{aligned} \quad (2.2)$$

where  $N(t)$  is the number of nodes at time  $t$ ,  $\Pi_O(k_O, t)$  is the probability that a node with observed degree  $k_O$  gains a new edge, and  $p_O(k_O, t)$  is the degree distribution. The first line corresponds to nodes whose observed degree remains unchanged from  $t$  to  $t+1$ , the first and second terms on the second line correspond to the transitions  $k_O - 1 \rightarrow k_O$  and  $k_O \rightarrow k_O + 1$  respectively, and the final term corresponds to the probability that the newly added node has initial degree  $k_O$ , given by  $p_H(k_O - 1)$ . Letting  $N(t) = t$  and assuming the degree distribution is stationary for large  $t$ ,

$$p_O(k_O) = \pi_O(k_O - 1) \cdot p_O(k_O - 1) - \pi_O(k_O) \cdot p_O(k_O) + 2^{1-k_O}, \text{ for } k \geq 2, \quad (2.3)$$

where

$$\pi_O(k_O) = t \cdot \Pi_O(k_O) = t \cdot \frac{1 + \langle k_H | k_O \rangle}{t} = 1 + \langle k_H | k_O \rangle, \quad (2.4)$$

and  $\langle k_H | k_O \rangle$  is the average degree of nodes in the hidden network with a fixed observed degree of  $k_O$ . Here, the  $1/t$  term corresponds to the probability that edges are gained from direct attachment, whereas the  $\langle k_H | k_O \rangle/t$  corresponds to the probability that edges are gained from copying.

## 2.2 Derivation of Eq. (9)

We would like to derive Eq. (9) in the main paper.

Consider the node  $\alpha$  added to the network at time  $t_\alpha$ . The initial conditions for node  $\alpha$  are

$$(k_H(t_\alpha))_\alpha = 1, \quad (2.5a)$$

$$\langle k_O(t_\alpha) \rangle_\alpha = 1 + \langle k_H(t_\alpha - 1) \rangle_\beta, \quad (2.5b)$$

where the final term is the average hidden degree of the target node  $\beta$ . In the hidden network, node  $\alpha$  gains edges from direct attachment only. Hence, at  $t > t_\alpha$ ,

$$\langle k_H(t > t_\alpha) \rangle_\alpha = 1 + \sum_{j=t_\alpha}^{t-1} \frac{1}{j} = 1 + H_{t-1} - H_{t_\alpha-1}, \quad (2.6)$$

where  $H_n$  is the  $n^{\text{th}}$  harmonic number. In the observed network, either node  $\alpha$  is targeted via direct attachment, or a copied edge is formed from the new node to node  $\alpha$  via any of the  $(k_H(t))_\alpha$  neighbours of node  $\alpha$ . Hence,

$$\langle k_O(t > t_\alpha) \rangle_\alpha = \langle k_O(t_\alpha) \rangle_\alpha + \sum_{j=t_\alpha}^{t-1} \frac{1 + \langle k_H(j) \rangle_\alpha}{j} = \langle k_O(t_\alpha) \rangle_\alpha + \sum_{j=t_\alpha}^{t-1} \frac{2 + H_j - H_{t_\alpha-1} - 1/j}{j}, \quad (2.7)$$

where we have subbed in Eq. (2.6) and  $H_{j-1} = H_j - 1/j$ . Note that

$$\sum_{j=1}^n \frac{H_j}{j} = \frac{1}{2} [(H_n)^2 + H_n^{(2)}], \quad (2.8)$$

where  $H_n^{(m)}$  is the  $n^{\text{th}}$  generalised Harmonic number of order  $m$  defined as

$$H_n^{(m)} = \sum_{j=1}^n \frac{1}{j^m}. \quad (2.9)$$

Hence, we can rewrite Eq. (2.7) as

$$\langle k_O(t > t_\alpha) \rangle_\alpha = \langle k_O(t_\alpha) \rangle_\alpha + (2 - H_{t_\alpha-1}) \sum_{j=t_\alpha}^{t-1} \frac{1}{j} + \sum_{j=t_\alpha}^{t-1} \frac{H_j}{j} - \sum_{j=t_\alpha}^{t-1} \frac{1}{j^2}, \quad (2.10)$$

which expanded gives

$$\begin{aligned} \langle k_O(t > t_\alpha) \rangle_\alpha &= \langle k_O(t_\alpha) \rangle_\alpha + (2 - H_{t_\alpha-1})(H_{t-1} - H_{t_\alpha-1}) \\ &\quad + \frac{1}{2} \left[ (H_{t-1})^2 + H_{t-1}^{(2)} - (H_{t_\alpha-1})^2 - H_{t_\alpha-1}^{(2)} \right] - (H_{t-1}^{(2)} - H_{t_\alpha-1}^{(2)}). \end{aligned} \quad (2.11)$$

We can simplify Eq. (2.11) slightly

$$\begin{aligned} \langle k_O(t > t_\alpha) \rangle_\alpha &= \langle k_O(t_\alpha) \rangle_\alpha + (2 - H_{t_\alpha-1})(H_{t-1} - H_{t_\alpha-1}) \\ &\quad + \frac{1}{2} \left[ (H_{t-1} + H_{t_\alpha-1})(H_{t-1} - H_{t_\alpha-1}) - H_{t-1}^{(2)} + H_{t_\alpha-1}^{(2)} \right], \end{aligned} \quad (2.12)$$

followed by

$$\langle k_O(t > t_\alpha) \rangle_\alpha = \langle k_O(t_\alpha) \rangle_\alpha + \frac{1}{2} \left[ (4 + H_{t-1} - H_{t_\alpha-1})(H_{t-1} - H_{t_\alpha-1}) - H_{t-1}^{(2)} + H_{t_\alpha-1}^{(2)} \right], \quad (2.13)$$

as required.
